# Supplementary material for: Learning Deterministic Weighted Automata with Queries and Counterexamples
Source: arXiv:1910.13895 source file (2019-12-29)
Supplement: Supplementary file 1 [file appendix_sample.tex]

\section{Sample Based PDFA Extraction}\label{App:Sample}
We adapt the sample based PDFA extraction algorithm given in ~\cite{PDFAClarkThollard2004} to take advantage of the direct queries made possible by extracting from an RNN.
Our adaptation changes the sampling method, and the implementation of anytime stopping. 
We do not directly use the RNN's probability for a given sequence when comparing states, as it raises other questions -- such as how to efficiently compare two states that have different sample sets. We leave a more thoughtful adaptation of these methods to future work.

\emph{Sampling} In the original method, transitions are processed by sampling the overall distribution until a single candidate state is reached by at least $m_0$ samples. In our adaptation we pick at each step the highest-probability candidate state, and sample the RNN $m_0$ times directly from its prefixes (proportionally to their probabilities). 

\emph{Unfinished Transitions} Where the original method maps unfinished transitions to a single 'ground state' at termination,
our adaptation can sample them directly and map them to the closest fit.
